# Supplementary material for: Metric Learning With HORDE: High-Order Regularizer for Deep Embeddings
Source: arXiv:1908.02735 source file (2019-08-07)
Supplement: Supplementary file 1 [file supplementary.tex]

\section{Learning rate}
    We try to learning rates : $10^{-5}$ and $10^{-6}$.
    In practice, all baselines are trained with a learning rate of $10^{-6}$ as they tend to diverge with the learning rate at $10^{-5}$.
    For all of our models, we use the learning rate of $10^{-5}$ which this time do not diverge and greatly speedup the training procedure for the same final performances.
    
\section{Precision on method}
%  From a domain adaptation point of view, the CNN representations $\vx_q$, $\vx_p$ and $\vx_n$ have distribution $\mathcal{I}_q$, $\mathcal{I}_p$ and $\mathcal{I}_n$ and we want to minimize the discrepancy between $\mathcal{I}_q$ and $\mathcal{I}_p$ as they belong to the same instance, and to maximize it between $\mathcal{I}_q$ and $\mathcal{I}_n$.
%  These distributions may be estimated using for example Gaussian Mixture Models, however, this method introduces a non-negligible offline computation that is sub-efficient as the properties of these distribution could change in each step of the training procedure.
 
%  Consequently, we propose to estimate these distributions by making the assumption that each distribution can be uniquely defined by its moments, and we present how to integrate such hypothesis into the deep metric learning framework.

\section{Proof}
